# Supplementary material for: Deep incremental learning models for financial temporal tabular datasets with distribution shifts
Source: arXiv:2303.07925 source file (2023-10-10)
Supplement: Supplementary file 1 [file additionalresults.tex]

\MB{This is the discussion about comparisons to other ML methods. If at all, it could go somewhere in the Discussion}

\begin{color}{magenta}

\subsection{Connections with common machine learning tasks}

The IL model presented above is a complete end-to-end autoML tool which transforms the given features into predictions. Different machine learning tasks, such as feature engineering and model stacking are integrated within the model. A key insight is that tabular models such as GBDT or MLP can be used repeatedly in different layers of the model to achieve the purpose of different machine learning tasks, which were previously considered separate tasks. Using just two building blocks, GBDT and MLP models, very complex and effective IL models can be built.

\paragraph{Feature Engineering/Selection} 

Feature Engineering is an important part of modelling tabular data. A wide range of standard feature engineering methods, including random non-linear transforms \cite{Horn19} and data-based methods such as feature tools \cite{James15} are proposed to learn higher-order feature relationships. Standard tabular models are then trained on the original features with the newly created features. More recent methods would use deep learning methods, in particular sequential attention for feature selection and engineering, examples include TabNet\cite{Arik_Pfister_2021} and TabTransformer \cite{TabTransformer}. For these models, feature engineering and tabular data modelling are performed in a single model. A major limitation of these models is high (active) memory consumption during model training. Another limitation is that many feature engineering methods are developed for \textit{static} datasets which assumes a set of relationships can be learnt on \textit{fixed} training set and then generalises to the test set. Unless these feature engineering components are retrained regularly as the downstream tabular models, the learnt relationships might not hold over distribution shifts of data. Most feature engineering methods applied to tabular data are a transformation from tabular features to another set of tabular features and are not much different than a collection of weakly trained tabular models. Under the IL framework, predictions from shallow trees and networks in the early layers can be considered as new features generated for downstream layers. It is not strictly necessary to make a distinction between feature engineering and tabular modelling. Training models in a multi-step layered structure avoids the look-ahead bias issue naturally.  Feature selection can be considered a special case of feature engineering where the feature engineering transformation to be learnt is a Boolean mask.

\paragraph{Feature Projection} 

Feature projection and its dynamic variant (Dynamic Feature Projection) introduced in the previous Numerai study \cite{wong2023online} can also be reformulated under the IL framework as follows. 

The need of feature projection is based on the assumption that unconstrained model training methods will result in model predictions that are explained by a small subset of features. While these models work well under data regimes that are similar to the training set, these models will suffer when there are distributional shifts in data. In investment terminology, unconstrained models are like investment portfolios concentrated in a small amount of assets, and therefore carry high risks under changes of market regimes. Feature projection, which can be used to limit both the maximal feature concentration risks and (linear)-dependencies of the model on the selected features can mitigate the impact of data distributional shifts by both spreading the model risk across a wider range of features and focusing more on the non-linear relationships between features. Dynamic feature projection suggests for data streams with distributional shifts, the optimal subset of features for projection is \textit{dynamic} rather than \textit{fixed}.  

A key issue that remained unresolved in the previous study \cite{wong2023online} is that the degree of feature projection and the size of the subset of features to be projected is given by useful heuristics, rather than being optimised based on data available. Clearly, these parameters can be learned from the dataset and adjusted according to data distribution shifts. Under the IL model, model predictions undergoing different feature projection processes can be combined in later layers. The optimal degree of feature projection depends on both the feature correlation structure and the target construction process.

\paragraph{Advanced Architectures of neural networks} 

Many advanced architectures of neural networks outperform basic multi-layer perceptron networks \cite{Arik_Pfister_2021,NODE,TabTransformer,} on a small amount of datasets presented in the research, which all of the datasets studied are \textit{static} machine learning problems. However, some research suggest the contrary when running the models using different hyperparameters or on \textit{different} datasets \cite{Arlind21,Leo22,Shwartz21}. As a result, the decision of whether advanced architectures are better than standard MLP for IL tasks on tabular datasets remains an open problem. 

For most IL problems, the only purpose is to generate high-quality and robust forecasts on \textit{future} observations using models trained on \textit{past} data only. A good performance based on \textit{historical} data is not relevant if the backtest performances cannot carry on into the future. An inherent limitation in interpreting research results from machine learning on temporal-based datasets is that results reported in a published journal article are only a \textit{snapshot} on the underlying data stream. When there are significant distribution shifts in data, conclusions can become invalid on new data arrived. This is a particular concern for neural networks models, which demonstrated high sensitivity to random seeds and training hyperparameters. 

Another limitation of deep learning methods with advanced architectures is that they are inherently difficult to interpret. Compared with the IL framework presented here, our model combines standalone ML models in a \textit{component-wise} manner, such that each component model can be evaluated independently and then inspected to monitor the changes in prediction quality in different layers. 

\paragraph{Model Stacking/Selection}

Stacking is a simple but highly effective technique to combine different ML model predictions. The concept of stacking is not limited to machine learning. In finance, portfolio optimisation are studied in detail to improve investment returns, where a convex optimisation is solved at each time step to find the linear combination of assets or strategies that maximise risk-adjusted return.

Under the IL framework, model stacking can be performed dynamically, which combined predicted ranking from different ML models at each era with different weights. Instead of considering model stacking as a \textit{separate} step to model training, model stacking can be incorporated as an extra layer in the IL model.

\end{color}

\MB{End of import}

%%% Feature Subsampling 

\paragraph{Deep XGBoost ensembles with different feature sampling methods}

While models trained with only a subset of features will have poorer performances than models trained with all the features. There are various reasons why we would want to train those less ideal models.

Feature subsampling can be used to simulate practical constraints in running a multi-strategy hedge fund, where data sharing between different teams are limited (due to legal or operational reasons). Each team would build strategies using a limited amount of data, with varying degree of overlapping knowledge with other teams. The strategies from each team are then combined at the fund level in a single portfolio. Indeed, feature subsampling can be used to generate a bootstrap estimate on the potential of strategy improvement if new data sources are added to the signal generation process. The improvement from individual models trained on only a subset of data to the ensemble model can be used to estimate the gap between the current trading model and the ideal portfolio trained with perfect knowledge. 

Feature subsampling are also effective ways to overcome hardware limitations in model training. Instead of training models using the whole dataset, which could be impossible due to memory constraints, we can use deep incremental learning to train models using subsets of features and then combine the predictions.

50 XGBoost models are trained with 10 different feature sampling schemes. In each sampling scheme, we randomly sample $50\%$ features globally and then train 5 models with different random seeds. The train size is fixed at 585 and the models are retrained every 50 eras. 

Other hyperparameters of the XGBoost models are set as follows. 

\begin{itemize}
    \item Grow policy: Depth-wise
    %\item Number of boosting rounds: 5000
    %\item Early Stopping 250
    %\item Learning rate: 0.01
    \item Max Depth: 4 
    %\item Max Leaves: 128 
    \item Min Samples per node: 10 
    \item Data subsample: 0.75
    \item Feature subsample by tree: 0.75
    \item Feature subsample by level/node: 1
    \item L1 regularisation: 0
    \item L2 regularisation: 0 
\end{itemize}

A deep XGBoost model is created by combining the 50 models incrementally. For every 10th era, a shallow XGBoost model with the following hyperparameters is trained using model predictions from the most recent 185 eras (with suitable data lag). Monotonic constraints are imposed so that we do not assign negative weights to the model predictions. This is repeated over 5 times over different random seeds.

%% Layer 2 XGBoost 
\begin{itemize}
    \item Grow policy: Depth-wise
    \item Number of boosting rounds: 20
    \item Early Stopping 20
    \item Learning rate: 0.1
    \item Max Depth: 4 
    %\item Max Leaves: 128 
    \item Min Samples per node: 10 
    \item Data subsample: 0.75
    \item Feature subsample by tree: 0.75
    \item Feature subsample by level/node: 1
    \item L1 regularisation: 0
    \item L2 regularisation: 0 
\end{itemize}

XGBoost models are trained with early-stopping for different number of boosting rounds and learning rates for 5 different random seeds. Three scenarios are considered: 
\begin{itemize}
    \item Small:    XGBoost models with 500 boosting rounds and learning rate 0.1, early-stopping at 25 rounds
    \item Standard: XGBoost models with 5000 boosting rounds and learning rate 0.01, early-stopping at 250 rounds
    \item Large:    XGBoost models with 50000 boosting rounds and learning rate 0.001, early-stopping at 2500 rounds
\end{itemize}
The 10 features sets are fixed across the scenarios.

In Table\ref{table:XGBFeature}, the performance of XGBoost models in Layer 1 of each sampling method are reported with the average over all the sampling methods (Average). The test period reported is Era 901 to Era 1050. We compare the deep XGBoost models in Layer 2 (Deep Incremental) with dynamic model selection from our previous study \cite{wong2023online,} (Dynamic Best), which selected the top 10 models (out of 50) based on recent performances. The criteria to select models is based on the highest Exponential Weighted Moving Averages (EWMA) Mean Corr with a weight decay of 0.001. Each selected top models have equal contribution.

Studying the joint effect of random feature selection and random seeds in training, we found that for some feature sets (Feature Set 3 for standard and large XGBoost models) have a much higher variance across random seeds than other feature sets. This effect is more readily observed for large XGBoost models, where all feature sets except Feature Set 3 have a variance smaller than 0.002 with the variance from Feature Set 3 being an outlier (0.0015). Therefore, it is important to repeat experiments using different random seeds over different steps of model learning. 

The feature sets with good performances for XGBoost models from smaller sizes does not generalise towards XGBoost models of larger sizes. The top 3 sets of small XGBoost models are from Feature Set 3,8,9. The top 3 sets of standard XGBoost models are from Feature Set 1,4,9. The top 3 sets of large XGBoost models are from Feature Set 1,4,9. The alignment of ranking of feature sets between standard and large XGBoost models are higher due to convergence of training process, as demonstrated in Figure \ref{figure/chapter3/XGBSnapshotPlot.pdf}. It demonstrated the joint effects between feature selection and training process. Variance between models with different feature sampling schemes decreases as the size of XGBoost models increases as expected. %The small XGBoost models have the highest variance between feature sets (0.001), where the standard and large XGBoost models have a lower variance between feature sets (0.0007,0.0008). 

Dynamic model selection created ensembles with a better Sharpe and Calmar ratio with Mean Corr not much significant different from the average over all feature sets (Average). Dynamic model selection provided good risk adjusted return but being over conservative in the test period.

Deep IL improves all three performances measures (Mean Corr, Sharpe and Calmar ratio) in the three scenarios. Deep IL models have a higher Mean Corr than dynamic model selection in all three scenarios. There are no significant differences of the Sharpe and Calmar ratios between deep IL models and dynamically selected models. 

Overall, deep IL achieves a well-rounded improvement in both absolute and risk-adjusted(relative) performance measures. 

\begin{table}[!ht]
 (a) Small XGBoost models (Max Boosting rounds = 500, Learning rate = 0.1)
\begin{center}
    \begin{tabular}{|l|l|l|l|}
        \hline
        Feature Set & Mean Corr & Sharpe & Calmar \\ \hline
        1  & 0.0181 $\pm$ 0.0011 & 0.8528 $\pm$ 0.0874 & 0.1617 $\pm$ 0.0550 \\ \hline
        2  & 0.0183 $\pm$ 0.0022 & 0.8692 $\pm$ 0.1043 & 0.1677 $\pm$ 0.0756 \\ \hline
        3  & 0.0182 $\pm$ 0.0024 & 0.9210 $\pm$ 0.1257 & 0.2088 $\pm$ 0.0691 \\ \hline
        4  & 0.0197 $\pm$ 0.0009 & 0.9896 $\pm$ 0.0641 & 0.1874 $\pm$ 0.0334 \\ \hline
        5  & 0.0180 $\pm$ 0.0024 & 0.8893 $\pm$ 0.1383 & 0.1686 $\pm$ 0.0511 \\ \hline
        6  & 0.0189 $\pm$ 0.0017 & 0.9518 $\pm$ 0.0973 & 0.2295 $\pm$ 0.0461 \\ \hline
        7  & 0.0180 $\pm$ 0.0014 & 0.8977 $\pm$ 0.0832 & 0.1903 $\pm$ 0.0450 \\ \hline
        8  & 0.0193 $\pm$ 0.0021 & 0.9428 $\pm$ 0.1353 & 0.1884 $\pm$ 0.0716 \\ \hline
        9  & 0.0201 $\pm$ 0.0011 & 0.9950 $\pm$ 0.0639 & 0.3160 $\pm$ 0.0962 \\ \hline
        10 & 0.0184 $\pm$ 0.0013 & 0.9484 $\pm$ 0.0608 & 0.1868 $\pm$ 0.0221 \\ \hline
        Average          & 0.0187  $\pm$ 0.0008    & 0.9257 $\pm$  0.0483 & 0.2005 $\pm$  0.0453 \\ \hline
        \hline 
        Deep Incremental & 0.0232   $\pm$  0.0004    & 1.1238 $\pm$  0.0167 & 0.2251  $\pm$  0.0073 \\ \hline
        Dynamic Best\cite{wong2023online}     & 0.0184        & 1.0174   & 0.1943   \\ \hline
        % Equal Weighted & 0.0240 & 1.0641 & 0.2132   \\ \hline
    \end{tabular}

\end{center}
\bigskip
(b) Standard XGBoost models (Max Boosting rounds = 5000, Learning rate = 0.01)
\begin{center}
%    \caption{Standard XGBoost models with different feature sampling schemes (5000 boosting rounds) }
    \begin{tabular}{|l|l|l|l|}
        \hline
        Feature Set      & Mean Corr  & Sharpe & Calmar  \\ \hline
        1  & 0.0238 $\pm$ 0.0008 & 1.0978 $\pm$ 0.0323 & 0.2418 $\pm$ 0.0170 \\ \hline
        2  & 0.0230 $\pm$ 0.0014 & 1.0824 $\pm$ 0.0886 & 0.2439 $\pm$ 0.0742 \\ \hline
        3  & 0.0214 $\pm$ 0.0027 & 1.0006 $\pm$ 0.1612 & 0.2512 $\pm$ 0.0739 \\ \hline
        4  & 0.0237 $\pm$ 0.0003 & 1.1711 $\pm$ 0.0168 & 0.2838 $\pm$ 0.0248 \\ \hline
        5  & 0.0233 $\pm$ 0.0005 & 1.1419 $\pm$ 0.0285 & 0.3261 $\pm$ 0.0343 \\ \hline
        6  & 0.0233 $\pm$ 0.0006 & 1.1215 $\pm$ 0.0246 & 0.3540 $\pm$ 0.0388 \\ \hline
        7  & 0.0224 $\pm$ 0.0001 & 1.1137 $\pm$ 0.0218 & 0.3481 $\pm$ 0.0486 \\ \hline
        8  & 0.0227 $\pm$ 0.0005 & 1.0866 $\pm$ 0.0281 & 0.2465 $\pm$ 0.0275 \\ \hline
        9  & 0.0237 $\pm$ 0.0003 & 1.1277 $\pm$ 0.0261 & 0.4895 $\pm$ 0.0581 \\ \hline
        10 & 0.0223 $\pm$ 0.0005 & 1.0851 $\pm$ 0.0485 & 0.3852 $\pm$ 0.0805 \\ \hline
        Average          & 0.0230    $\pm$  0.0008    & 1.1028 $\pm$  0.0456 & 0.3170 $\pm$  0.0804 \\ \hline
        \hline 
        Deep Incremental & 0.0238    $\pm$  0.0002    & 1.1434 $\pm$  0.0165 & 0.3454 $\pm$  0.0410 \\ \hline
        Dynamic Best\cite{wong2023online}     & 0.0231     & 1.1671    & 0.3022    \\ \hline
        % Equal Weighted & 0.0246 & 1.1483 & 0.3273   \\ \hline
    \end{tabular}

\end{center}
\bigskip
(c) Large XGBoost models (Max Boosting rounds = 50000, Learning rate = 0.001)
\begin{center}
%    \caption{Large XGBoost models with different feature sampling schemes (50000 boosting rounds) }
    \begin{tabular}{|l|l|l|l|l|l|l|}
        \hline
        Feature Set      & Mean Corr  & Sharpe & Calmar  \\ \hline
        1  & 0.0241 $\pm$ 0.0002 & 1.1148 $\pm$ 0.0146 & 0.2847 $\pm$ 0.0074 \\ \hline
        2  & 0.0232 $\pm$ 0.0002 & 1.1063 $\pm$ 0.0119 & 0.3063 $\pm$ 0.0197 \\ \hline
        3  & 0.0213 $\pm$ 0.0026 & 0.9824 $\pm$ 0.1529 & 0.2642 $\pm$ 0.0754 \\ \hline
        4  & 0.0243 $\pm$ 0.0002 & 1.2043 $\pm$ 0.0138 & 0.3074 $\pm$ 0.0126 \\ \hline
        5  & 0.0241 $\pm$ 0.0002 & 1.1748 $\pm$ 0.0082 & 0.3178 $\pm$ 0.0156 \\ \hline
        6  & 0.0235 $\pm$ 0.0002 & 1.1323 $\pm$ 0.0125 & 0.4130 $\pm$ 0.0100 \\ \hline
        7  & 0.0223 $\pm$ 0.0001 & 1.0952 $\pm$ 0.0114 & 0.3736 $\pm$ 0.0147 \\ \hline
        8  & 0.0232 $\pm$ 0.0003 & 1.1150 $\pm$ 0.0157 & 0.2686 $\pm$ 0.0067 \\ \hline
        9  & 0.0239 $\pm$ 0.0003 & 1.1376 $\pm$ 0.0149 & 0.5036 $\pm$ 0.0251 \\ \hline
        10 & 0.0223 $\pm$ 0.0002 & 1.0882 $\pm$ 0.0184 & 0.4069 $\pm$ 0.0169 \\ \hline
        Average          & 0.0232    $\pm$  0.0010    & 1.1151 $\pm$  0.0588 & 0.3446 $\pm$  0.0775 \\ \hline
        \hline 
        Deep Incremental & 0.0236    $\pm$  0.0003   & 1.1505 $\pm$  0.0248 & 0.4147 $\pm$  0.0350 \\ \hline
        Dynamic Best\cite{wong2023online}     & 0.0233       & 1.1406   & 0.3398    \\ \hline
        % Equal Weighted  & 0.0244 & 1.1413 & 0.3591 \\ \hline 
    \end{tabular}
\end{center}
\smallskip
    \caption{Performance of (a) small, (b) standard and (c) large XGBoost Models with different feature sampling schemes on test period  (Eras 901-1050)}
    \label{table:XGBFeature}
\end{table}

%%% Old Way of Feature Projecting based on bad XGBoost Features 

\paragraph{Projecting bad XGBoost features} 

In \cite{wong2023online}, dynamic feature projection was used to project bad features from model predictions as a mitigation against regime changes in data and reduce drawdown of trading strategies. Instead of using the recent performances of features to decide which features are bad, feature importance from IL XGBoost models, which are dynamically constructed as the models are retrained can be used to filter bad features for projection. Here, we define feature importance based on the number of times a feature is used to split the data across all trees in the XGBoost model. 

There are two reasons why we do not use the feature performances as in \cite{wong2023online} to select the subset of bad features for projection. The first is because the IL XGBoost models are already dynamically updated, which means the models are always using the features that are important within the most recent lookback window in building the trees. It is a duplication of effort in trying to calculate the feature performances, based on linear correlation again, since XGBoost already done that in a better way which taken into account both linear and non-linear relationships. The second is for computational reasons, as reusing the information captured in the training of XGBoost models means there is no additional computational costs to compute the feature performances (correlations) as in \cite{wong2023online}.

In the following, we will project bad features suggested by XGBoost models, which are the least used $10\%$ features in splitting. We compare our dynamic feature projection, based on bad XGBoost models, with the baseline selection method using the 416 features recommend by Numerai \cite{numerai-datav4.1} \footnote{In older versions of data, 420 features are recommend by Numerai for feature projection. 4 features are removed due to data quality of issues}.

We then proceed to train XGBoost models with 10 different feature sampling scheme.In each sampling scheme, we randomly sample $50\%$ features from the 1586 features globally for model training.

%% Results of 
In the validation period, feature projection can improve Calmar ratios significantly but the impact is less significant in the test period.

Repeating the experiments on XGBoost models trained without early stopping, we do not see the improvement of Calmar ratio in the test period for the large XGBoost models. 

%% Discussion
Feature importance from XGBoost models trained with early stopping are informative to indicate the quality of features. As early stopping

%% Test Period Ensemble 

\begin{table}[]
\begin{tabular}{|c|c|c|l|l|l|}
\hline
Feature Set     &  Ensemble   & Projection  & Mean Corr & Sharpe & Calmar \\ \hline
\multirow{6}{*}{Small}  & \multirow{2}{*}{Deep Incremental}   & No     & 0.0232   $\pm$  0.0004    & 1.1238 $\pm$  0.0167 & 0.2251  $\pm$  0.0073 \\ \cline{3-6}
                        &                                     & XGB    & 0.0214 $\pm$ 0.003 & 1.1158 $\pm$ 0.0285 & 0.4963 $\pm$ 0.0921  \\ \cline{2-6}
                        & \multirow{2}{*}{Dynamic Best\cite{wong2023online}}  & No  & 0.0184        & 1.0174   & 0.1943   \\ \cline{3-6}
                        &                                     & XGB    & 0.0133 & 1.0609 & 0.5774 \\ \cline{2-6}
                        & \multirow{2}{*}{Equal Weighted}  & No  & 0.0240 & 1.0641 & 0.2132  \\ \cline{3-6}
        &                                     & XGB   & 0.0216 & 1.0792 & 0.2544 \\ \hline                   
\multirow{6}{*}{Standard}  & \multirow{2}{*}{Deep Incremental}   & No     & 0.0238    $\pm$  0.0002    & 1.1434 $\pm$  0.0165 & 0.3454 $\pm$  0.0410 \\ \cline{3-6}
                        &                                     & XGB   & 0.0219    $\pm$  0.0004    & 1.0962 $\pm$  0.0191 & 0.2906 $\pm$  0.0206 \\ \cline{2-6}
                        & \multirow{2}{*}{Dynamic Best\cite{wong2023online}}  & No & 0.0231     & 1.1671    & 0.3022  \\ \cline{3-6}
                        &                                     & XGB   & 0.0200 & 1.1734 & 0.4032 \\ \cline{2-6}
                        & \multirow{2}{*}{Equal Weighted}  & No & 0.0246 & 1.1483 & 0.3273  \\ \cline{3-6}
                        &                                     & XGB   & 0.0221 & 1.1496 & 0.3782 \\ \hline                     
\multirow{6}{*}{Large}  & \multirow{2}{*}{Deep Incremental}   & No     & 0.0236    $\pm$  0.0003   & 1.1505 $\pm$  0.0248 & 0.4147 $\pm$  0.0350  \\ \cline{3-6}
                        &                                     & XGB   & 0.0215 $\pm$ 0.0004 & 1.1049 $\pm$ 0.0288 & 0.4861 $\pm$ 0.0298 \\ \cline{2-6}
                        & \multirow{2}{*}{Dynamic Best\cite{wong2023online}}  & No  & 0.0233       & 1.1406   & 0.3398 \\ \cline{3-6}
                        &                                     & XGB  & 0.0211 & 1.1988 & 0.5348 \\ \cline{2-6}
                        & \multirow{2}{*}{Equal Weighted}  & No & 0.0244 & 1.1413 & 0.3591 \\ \cline{3-6}
                        &                                     & XGB   & 0.0224 & 1.1732 & 0.4395 \\ \hline                        
\end{tabular}
\smallskip
    \caption{Performance of ensemble XGBoost Models with different feature sampling schemes and feature projection schemes (No: No feature projection, XGB: Bad features based on XGBoost feature importance,) on test period  (Eras 901-1050)}
    \label{table:XGBFeatureEnsemble-test}
\end{table}

%%% Test Period, Feature Projection

\begin{table}[]
\begin{tabular}{|c|c|l|l|l|}
\hline
Feature Set         & Projection  & Mean Corr & Sharpe & Calmar \\ \hline
\multirow{3}{*}{1}              & No                       & 0.0180 $\pm$ 0.0011 & 0.8528 $\pm$ 0.0875 & 0.1617 $\pm$ 0.0550 \\ \cline{2-5}
                                & XGB                    & 0.0132 $\pm$ 0.0017 & 0.7531 $\pm$ 0.0903 & 0.2241 $\pm$ 0.1034 \\ \cline{2-5}
                                & Numerai                    & 0.0099 $\pm$ 0.0016 & 0.5835 $\pm$ 0.1241 & 0.0584 $\pm$ 0.0231 \\ \hline
\multirow{3}{*}{2}              & No                       & 0.0183 $\pm$ 0.0022 & 0.8692 $\pm$ 0.1043 & 0.1677 $\pm$ 0.0756 \\ \cline{2-5}
                                & XGB                    & 0.0136 $\pm$ 0.0021 & 0.8134 $\pm$ 0.0980 & 0.1805 $\pm$ 0.1078 \\ \cline{2-5}
                                & Numerai                    & 0.0099 $\pm$ 0.0015 & 0.5996 $\pm$ 0.0783 & 0.0657 $\pm$ 0.0173 \\ \hline
\multirow{3}{*}{3}              & No                       & 0.0182 $\pm$ 0.0024 & 0.9210 $\pm$ 0.1257 & 0.2088 $\pm$ 0.0691 \\ \cline{2-5}
                                & XGB                    & 0.0133 $\pm$ 0.0027 & 0.7869 $\pm$ 0.1708 & 0.2330 $\pm$ 0.2275 \\ \cline{2-5}
                                & Numerai                    & 0.0099 $\pm$ 0.0019 & 0.5767 $\pm$ 0.1245 & 0.0633 $\pm$ 0.0346 \\ \hline
\multirow{3}{*}{4}              & No                       & 0.0197 $\pm$ 0.0009 & 0.9896 $\pm$ 0.0641 & 0.1874 $\pm$ 0.0334 \\ \cline{2-5}
                                & XGB                    & 0.0151 $\pm$ 0.0014 & 0.8802 $\pm$ 0.0464 & 0.1961 $\pm$ 0.0594 \\ \cline{2-5}
                                & Numerai                    & 0.0123 $\pm$ 0.0014 & 0.7183 $\pm$ 0.0514 & 0.0923 $\pm$ 0.0139 \\ \hline
\multirow{3}{*}{5}              & No                       & 0.0180 $\pm$ 0.0024 & 0.8892 $\pm$ 0.1383 & 0.1686 $\pm$ 0.0511 \\ \cline{2-5}
                                & XGB                    & 0.0144 $\pm$ 0.0023 & 0.7882 $\pm$ 0.1411 & 0.2172 $\pm$ 0.0677 \\ \cline{2-5}
                                & Numerai                    & 0.0101 $\pm$ 0.0021 & 0.5934 $\pm$ 0.1178 & 0.0637 $\pm$ 0.0089 \\ \hline
\multirow{3}{*}{6}              & No                       & 0.0189 $\pm$ 0.0017 & 0.9518 $\pm$ 0.0972 & 0.2295 $\pm$ 0.0461 \\ \cline{2-5}
                                & XGB                    & 0.0150 $\pm$ 0.0014 & 0.8748 $\pm$ 0.1049 & 0.2238 $\pm$ 0.0912 \\ \cline{2-5}
                                & Numerai                    & 0.0113 $\pm$ 0.0010 & 0.6888 $\pm$ 0.0760 & 0.0932 $\pm$ 0.0250 \\ \hline
\multirow{3}{*}{7}              & No                       & 0.0180 $\pm$ 0.0014 & 0.8977 $\pm$ 0.0832 & 0.1903 $\pm$ 0.0450 \\ \cline{2-5}
                                & XGB                    & 0.0137 $\pm$ 0.0027 & 0.7568 $\pm$ 0.1506 & 0.1335 $\pm$ 0.0643 \\ \cline{2-5}
                                & Numerai                    & 0.0096 $\pm$ 0.0019 & 0.5367 $\pm$ 0.0794 & 0.0412 $\pm$ 0.0029 \\ \hline
\multirow{3}{*}{8}              & No                       & 0.0193 $\pm$ 0.0021 & 0.9428 $\pm$ 0.1353 & 0.1884 $\pm$ 0.0716 \\ \cline{2-5}
                                & XGB                    & 0.0144 $\pm$ 0.0025 & 0.8420 $\pm$ 0.1537 & 0.1411 $\pm$ 0.0720 \\ \cline{2-5}
                                & Numerai                    & 0.0109 $\pm$ 0.0020 & 0.6176 $\pm$ 0.1323 & 0.0606 $\pm$ 0.0408 \\ \hline
\multirow{3}{*}{9}              & No                       & 0.0201 $\pm$ 0.0011 & 0.9950 $\pm$ 0.0639 & 0.3160 $\pm$ 0.0962 \\ \cline{2-5}
                                & XGB                    & 0.0138 $\pm$ 0.0016 & 0.7446 $\pm$ 0.1101 & 0.1580 $\pm$ 0.1065 \\ \cline{2-5}
                                & Numerai                    & 0.0117 $\pm$ 0.0018 & 0.6563 $\pm$ 0.1000 & 0.0658 $\pm$ 0.0180 \\ \hline
\multirow{3}{*}{10}             & No                       & 0.0184 $\pm$ 0.0013 & 0.9484 $\pm$ 0.0608 & 0.1868 $\pm$ 0.0221 \\ \cline{2-5}
                                & XGB                    & 0.0146 $\pm$ 0.0014 & 0.8385 $\pm$ 0.1088 & 0.1444 $\pm$ 0.0464 \\ \cline{2-5}
                                & Numerai                    & 0.0106 $\pm$ 0.0011 & 0.6377 $\pm$ 0.0799 & 0.0834 $\pm$ 0.0346 \\ \hline
\end{tabular}
\smallskip
    \caption{Performance of small XGBoost Models with different feature sampling schemes and feature projection schemes (No: No feature projection, XGB: Bad features based on XGBoost feature importance, Numerai: fixed set of 416 features given by Numerai) on test period  (Eras 901-1050)}
    \label{table:XGBFeatureSmall-test}
\end{table}

\begin{table}[]
\begin{tabular}{|c|c|l|l|l|}
\hline
Feature Set         & Projection  & Mean Corr & Sharpe & Calmar \\ \hline
\multirow{3}{*}{1}              & No                       & 0.0238 $\pm$ 0.0008 & 1.0978 $\pm$ 0.0323 & 0.2419 $\pm$ 0.0170 \\ \cline{2-5} 
                                & XGB                    & 0.0203 $\pm$ 0.0016 & 1.0880 $\pm$ 0.0618 & 0.3458 $\pm$ 0.0642 \\ \cline{2-5} 
                                & Numerai                    & 0.0163 $\pm$ 0.0009 & 0.8908 $\pm$ 0.0540 & 0.2338 $\pm$ 0.0656 \\ \hline
\multirow{3}{*}{2}              & No                       & 0.0230 $\pm$ 0.0014 & 1.0824 $\pm$ 0.0886 & 0.2439 $\pm$ 0.0742 \\ \cline{2-5} 
                                & XGB                    & 0.0185 $\pm$ 0.0010 & 1.0273 $\pm$ 0.1097 & 0.3461 $\pm$ 0.1969 \\ \cline{2-5} 
                                & Numerai                    & 0.0150 $\pm$ 0.0017 & 0.8164 $\pm$ 0.1012 & 0.1107 $\pm$ 0.0514 \\ \hline
\multirow{3}{*}{3}              & No                       & 0.0214 $\pm$ 0.0027 & 1.0006 $\pm$ 0.1612 & 0.2512 $\pm$ 0.0739 \\ \cline{2-5} 
                                & XGB                    & 0.0177 $\pm$ 0.0028 & 0.9597 $\pm$ 0.1706 & 0.2932 $\pm$ 0.1091 \\ \cline{2-5} 
                                & Numerai                    & 0.0142 $\pm$ 0.0023 & 0.7326 $\pm$ 0.1482 & 0.0682 $\pm$ 0.0284 \\ \hline
\multirow{3}{*}{4}              & No                       & 0.0237 $\pm$ 0.0003 & 1.1711 $\pm$ 0.0168 & 0.2839 $\pm$ 0.0248 \\ \cline{2-5} 
                                & XGB                    & 0.0208 $\pm$ 0.0004 & 1.1346 $\pm$ 0.0211 & 0.5206 $\pm$ 0.1292 \\ \cline{2-5} 
                                & Numerai                    & 0.0160 $\pm$ 0.0004 & 0.8411 $\pm$ 0.0351 & 0.1380 $\pm$ 0.0520 \\ \hline
\multirow{3}{*}{5}              & No                       & 0.0233 $\pm$ 0.0005 & 1.1419 $\pm$ 0.0285 & 0.3261 $\pm$ 0.0343 \\ \cline{2-5} 
                                & XGB                    & 0.0204 $\pm$ 0.0008 & 1.0860 $\pm$ 0.0514 & 0.3224 $\pm$ 0.0556 \\ \cline{2-5} 
                                & Numerai                    & 0.0153 $\pm$ 0.0005 & 0.8436 $\pm$ 0.0371 & 0.1023 $\pm$ 0.0115 \\ \hline
\multirow{3}{*}{6}              & No                       & 0.0233 $\pm$ 0.0007 & 1.1215 $\pm$ 0.0246 & 0.3540 $\pm$ 0.0387 \\ \cline{2-5} 
                                & XGB                    & 0.0191 $\pm$ 0.0011 & 0.9858 $\pm$ 0.0591 & 0.4068 $\pm$ 0.1227 \\ \cline{2-5} 
                                & Numerai                    & 0.0149 $\pm$ 0.0008 & 0.7779 $\pm$ 0.0305 & 0.0868 $\pm$ 0.0131 \\ \hline
\multirow{3}{*}{7}              & No                       & 0.0224 $\pm$ 0.0001 & 1.1137 $\pm$ 0.0218 & 0.3481 $\pm$ 0.0486 \\ \cline{2-5} 
                                & XGB                    & 0.0196 $\pm$ 0.0009 & 1.0348 $\pm$ 0.0432 & 0.3040 $\pm$ 0.0321 \\ \cline{2-5} 
                                & Numerai                    & 0.0155 $\pm$ 0.0007 & 0.8065 $\pm$ 0.0439 & 0.0774 $\pm$ 0.0088 \\ \hline
\multirow{3}{*}{8}              & No                       & 0.0227 $\pm$ 0.0005 & 1.0865 $\pm$ 0.0281 & 0.2465 $\pm$ 0.0275 \\ \cline{2-5} 
                                & XGB                    & 0.0187 $\pm$ 0.0010 & 0.9684 $\pm$ 0.0426 & 0.2950 $\pm$ 0.0588 \\ \cline{2-5} 
                                & Numerai                    & 0.0148 $\pm$ 0.0005 & 0.7778 $\pm$ 0.0167 & 0.0692 $\pm$ 0.0097 \\ \hline
\multirow{3}{*}{9}              & No                       & 0.0236 $\pm$ 0.0003 & 1.1277 $\pm$ 0.0261 & 0.4895 $\pm$ 0.0581 \\ \cline{2-5} 
                                & XGB                    & 0.0185 $\pm$ 0.0009 & 1.0174 $\pm$ 0.0646 & 0.3005 $\pm$ 0.1095 \\ \cline{2-5} 
                                & Numerai                    & 0.0169 $\pm$ 0.0003 & 0.8971 $\pm$ 0.0214 & 0.1206 $\pm$ 0.0121 \\ \hline
\multirow{3}{*}{10}             & No                       & 0.0223 $\pm$ 0.0005 & 1.0851 $\pm$ 0.0485 & 0.3852 $\pm$ 0.0805 \\ \cline{2-5} 
                                & XGB                    & 0.0184 $\pm$ 0.0006 & 0.9639 $\pm$ 0.0464 & 0.3715 $\pm$ 0.1005 \\ \cline{2-5} 
                                & Numerai                    & 0.0139 $\pm$ 0.0007 & 0.7344 $\pm$ 0.0285 & 0.0877 $\pm$ 0.0140 \\ \hline
\end{tabular}
\smallskip
    \caption{Performance of standard XGBoost Models with different feature sampling schemes and feature projection schemes (No: No feature projection, XGB: Bad features based on XGBoost feature importance, Numerai: fixed set of 416 features given by Numerai) on test period  (Eras 901-1050)}
    \label{table:XGBFeatureStandard-test}
\end{table}

\begin{table}[]
\begin{tabular}{|c|c|l|l|l|}
\hline
Feature Set         & Projection  & Mean Corr & Sharpe & Calmar \\ \hline
\multirow{3}{*}{1}  & No    & 0.0241   $\pm$ 0.0002    & 1.1148$\pm$ 0.0146    & 0.2847$\pm$ 0.0074    \\ \cline{2-5}
        & XGB & 0.0221   $\pm$ 0.0003    & 1.2098$\pm$ 0.0131    & 0.4983$\pm$ 0.1512    \\ \cline{2-5}
        & Numerai & 0.0164   $\pm$ 0.0003    & 0.8831$\pm$ 0.0160    & 0.2476$\pm$ 0.0236    \\ \hline
\multirow{3}{*}{2}  & No    & 0.0232   $\pm$ 0.0002    & 1.1062$\pm$ 0.0119    & 0.3063$\pm$ 0.0197    \\ \cline{2-5}
        & XGB & 0.0203   $\pm$ 0.0008    & 1.1653$\pm$ 0.0578    & 0.4174$\pm$ 0.0700    \\ \cline{2-5}
        & Numerai & 0.0154   $\pm$ 0.0002    & 0.8495$\pm$ 0.0073    & 0.1214$\pm$ 0.0045    \\ \hline
\multirow{3}{*}{3}  & No    & 0.0213   $\pm$ 0.0026    & 0.9824$\pm$ 0.1528    & 0.2642$\pm$ 0.0754    \\ \cline{2-5}
        & XGB & 0.0175   $\pm$ 0.0029    & 0.9220$\pm$ 0.1724    & 0.3475$\pm$ 0.1534    \\ \cline{2-5}
        & Numerai & 0.0147   $\pm$ 0.0018    & 0.7411$\pm$ 0.1162    & 0.0717$\pm$ 0.0151    \\ \hline
\multirow{3}{*}{4}  & No    & 0.0243   $\pm$ 0.0002    & 1.2043$\pm$ 0.0137    & 0.3074$\pm$ 0.0126    \\ \cline{2-5}
        & XGB & 0.0219   $\pm$ 0.0005    & 1.1771$\pm$ 0.0301    & 0.6554$\pm$ 0.1629    \\ \cline{2-5}
        & Numerai & 0.0164   $\pm$ 0.0003    & 0.8633$\pm$ 0.0178    & 0.1406$\pm$ 0.0090    \\ \hline
\multirow{3}{*}{5}  & No    & 0.0241   $\pm$ 0.0003    & 1.1748$\pm$ 0.0082    & 0.3178$\pm$ 0.0156    \\ \cline{2-5}
        & XGB & 0.0213   $\pm$ 0.0006    & 1.1059$\pm$ 0.0271    & 0.4596$\pm$ 0.0709    \\ \cline{2-5}
        & Numerai & 0.0161   $\pm$ 0.0002    & 0.8787$\pm$ 0.0193    & 0.1207$\pm$ 0.0086    \\ \hline
\multirow{3}{*}{6}  & No    & 0.0235   $\pm$ 0.0002    & 1.1323$\pm$ 0.0125    & 0.4130$\pm$ 0.0100    \\ \cline{2-5}
        & XGB & 0.0204   $\pm$ 0.0005    & 1.0461$\pm$ 0.0269    & 0.4857$\pm$ 0.0589    \\ \cline{2-5}
        & Numerai & 0.0158   $\pm$ 0.0003    & 0.8174$\pm$ 0.0151    & 0.1094$\pm$ 0.0084    \\ \hline
\multirow{3}{*}{7}  & No    & 0.0223   $\pm$ 0.0001    & 1.0952$\pm$ 0.0114    & 0.3736$\pm$ 0.0147    \\ \cline{2-5}
        & XGB & 0.0205   $\pm$ 0.0004    & 1.0411$\pm$ 0.0225    & 0.3645$\pm$ 0.0446    \\ \cline{2-5}
        & Numerai & 0.0163   $\pm$ 0.0002    & 0.8289$\pm$ 0.0115    & 0.0837$\pm$ 0.0034    \\ \hline
\multirow{3}{*}{8}  & No    & 0.0232   $\pm$ 0.0002    & 1.1150$\pm$ 0.0157    & 0.2686$\pm$ 0.0066    \\ \cline{2-5}
        & XGB & 0.0201   $\pm$ 0.0004    & 1.0400$\pm$ 0.0207    & 0.3917$\pm$ 0.0537    \\ \cline{2-5}
        & Numerai & 0.0160   $\pm$ 0.0003    & 0.8232$\pm$ 0.0210    & 0.0716$\pm$ 0.0050    \\ \hline
\multirow{3}{*}{9}  & No    & 0.0239   $\pm$ 0.0002    & 1.1376$\pm$ 0.0149    & 0.5036$\pm$ 0.0251    \\ \cline{2-5}
        & XGB & 0.0197   $\pm$ 0.0004    & 1.0487$\pm$ 0.0194    & 0.4342$\pm$ 0.0521    \\ \cline{2-5}
        & Numerai & 0.0174   $\pm$ 0.0003    & 0.9400$\pm$ 0.0217    & 0.1458$\pm$ 0.0019    \\ \hline
\multirow{3}{*}{10} & No    & 0.0223   $\pm$ 0.0002    & 1.0882$\pm$ 0.0184    & 0.4069$\pm$ 0.0169    \\ \cline{2-5}
        & XGB & 0.0187   $\pm$ 0.0004    & 1.0019$\pm$ 0.0541    & 0.3954$\pm$ 0.0735    \\ \cline{2-5}
        & Numerai & 0.0139   $\pm$ 0.0003    & 0.7273$\pm$ 0.0170    & 0.0843$\pm$ 0.0086    \\ \hline
\end{tabular}
\smallskip
    \caption{Performance of large XGBoost Models with different feature sampling schemes and feature projection schemes (No: No feature projection, XGB: Bad features based on XGBoost feature importance, Numerai: fixed set of 416 features given by Numerai) on test period  (Eras 901-1050)}
    \label{table:XGBFeatureLarge-test}
\end{table}

%% Validation period,  Feature Projection 

\begin{table}[]
\begin{tabular}{|c|c|l|l|l|}
\hline
Feature Set         & Projection  & Mean Corr & Sharpe & Calmar \\ \hline
\multirow{3}{*}{1}  & No     & 0.0199 $\pm$ 0.0014 & 1.0460 $\pm$ 0.0904 & 0.1470 $\pm$ 0.0519 \\ \cline{2-5} 
        & XGB        & 0.0190 $\pm$ 0.0019 & 1.0955 $\pm$ 0.1479 & 0.2519 $\pm$ 0.1089 \\ \cline{2-5} 
        & Numerai        & 0.0150 $\pm$ 0.0016 & 0.9436 $\pm$ 0.1184 & 0.2692 $\pm$ 0.0681 \\ \hline
\multirow{3}{*}{2}  & No     & 0.0201 $\pm$ 0.0014 & 1.0860 $\pm$ 0.0813 & 0.2553 $\pm$ 0.1505 \\ \cline{2-5} 
        & XGB        & 0.0181 $\pm$ 0.0012 & 1.0722 $\pm$ 0.0932 & 0.2752 $\pm$ 0.1380 \\ \cline{2-5} 
        & Numerai        & 0.0146 $\pm$ 0.0009 & 0.9519 $\pm$ 0.0762 & 0.2342 $\pm$ 0.0696 \\ \hline
\multirow{3}{*}{3}  & No     & 0.0198 $\pm$ 0.0008 & 1.0587 $\pm$ 0.0876 & 0.1452 $\pm$ 0.0424 \\ \cline{2-5} 
        & XGB        & 0.0179 $\pm$ 0.0004 & 1.0322 $\pm$ 0.0746 & 0.2436 $\pm$ 0.0667 \\ \cline{2-5} 
        & Numerai        & 0.0135 $\pm$ 0.0010 & 0.8388 $\pm$ 0.0710 & 0.2169 $\pm$ 0.0676 \\ \hline
\multirow{3}{*}{4}  & No     & 0.0219 $\pm$ 0.0010 & 1.1863 $\pm$ 0.0645 & 0.2026 $\pm$ 0.0510 \\ \cline{2-5} 
        & XGB        & 0.0199 $\pm$ 0.0011 & 1.1443 $\pm$ 0.0497 & 0.2083 $\pm$ 0.0284 \\ \cline{2-5} 
        & Numerai        & 0.0158 $\pm$ 0.0009 & 0.9982 $\pm$ 0.0846 & 0.2830 $\pm$ 0.0728 \\ \hline
\multirow{3}{*}{5}  & No     & 0.0202 $\pm$ 0.0011 & 1.0582 $\pm$ 0.0585 & 0.2108 $\pm$ 0.0457 \\ \cline{2-5} 
        & XGB        & 0.0187 $\pm$ 0.0007 & 1.0585 $\pm$ 0.0667 & 0.2487 $\pm$ 0.0876 \\ \cline{2-5} 
        & Numerai        & 0.0144 $\pm$ 0.0014 & 0.8805 $\pm$ 0.1189 & 0.2197 $\pm$ 0.1333 \\ \hline
\multirow{3}{*}{6}  & No     & 0.0208 $\pm$ 0.0009 & 1.1040 $\pm$ 0.0704 & 0.1481 $\pm$ 0.0699 \\ \cline{2-5} 
        & XGB        & 0.0189 $\pm$ 0.0009 & 1.1084 $\pm$ 0.0626 & 0.2886 $\pm$ 0.1490 \\ \cline{2-5} 
        & Numerai        & 0.0146 $\pm$ 0.0010 & 0.9640 $\pm$ 0.0967 & 0.2679 $\pm$ 0.1102 \\ \hline
\multirow{3}{*}{7}  & No     & 0.0198 $\pm$ 0.0006 & 1.0449 $\pm$ 0.0268 & 0.1649 $\pm$ 0.0533 \\ \cline{2-5} 
        & XGB        & 0.0180 $\pm$ 0.0005 & 1.0335 $\pm$ 0.0332 & 0.2411 $\pm$ 0.0543 \\ \cline{2-5} 
        & Numerai        & 0.0143 $\pm$ 0.0005 & 0.8842 $\pm$ 0.0575 & 0.1996 $\pm$ 0.0628 \\ \hline
\multirow{3}{*}{8}  & No     & 0.0217 $\pm$ 0.0013 & 1.1759 $\pm$ 0.0692 & 0.1873 $\pm$ 0.0273 \\ \cline{2-5} 
        & XGB        & 0.0192 $\pm$ 0.0017 & 1.1501 $\pm$ 0.1202 & 0.2712 $\pm$ 0.1396 \\ \cline{2-5} 
        & Numerai        & 0.0158 $\pm$ 0.0021 & 1.0226 $\pm$ 0.1374 & 0.3268 $\pm$ 0.1027 \\ \hline
\multirow{3}{*}{9}  & No     & 0.0204 $\pm$ 0.0009 & 1.0595 $\pm$ 0.0598 & 0.1886 $\pm$ 0.0631 \\ \cline{2-5} 
        & XGB        & 0.0181 $\pm$ 0.0009 & 1.0578 $\pm$ 0.0578 & 0.2526 $\pm$ 0.0680 \\ \cline{2-5} 
        & Numerai        & 0.0149 $\pm$ 0.0016 & 0.9128 $\pm$ 0.0650 & 0.1971 $\pm$ 0.0496 \\ \hline
\multirow{3}{*}{10} & No     & 0.0194 $\pm$ 0.0009 & 1.0013 $\pm$ 0.0418 & 0.1377 $\pm$ 0.0203 \\ \cline{2-5} 
        & XGB        & 0.0171 $\pm$ 0.0010 & 0.9849 $\pm$ 0.0647 & 0.1978 $\pm$ 0.0542 \\ \cline{2-5} 
        & Numerai        & 0.0134 $\pm$ 0.0010 & 0.8400 $\pm$ 0.0832 & 0.1864 $\pm$ 0.0482 \\ \hline
\end{tabular}
\smallskip
    \caption{Performance of small XGBoost Models with different feature sampling schemes and feature projection schemes (No: No feature projection, XGB: Bad features based on XGBoost feature importance, Numerai: fixed set of 416 features given by Numerai) on validation period (Eras 601-885)}
    \label{table:XGBFeatureSmall-validate}
\end{table}

\begin{table}[]
\begin{tabular}{|c|c|l|l|l|}
\hline
Feature Set         & Projection  & Mean Corr & Sharpe & Calmar \\ \hline
\multirow{3}{*}{1}   & No          & 0.0264 $\pm$ 0.0003 & 1.3907 $\pm$ 0.0215 & 0.2732 $\pm$ 0.0301 \\ \cline{2-5} 
          & XGB         & 0.0255 $\pm$ 0.0004 & 1.4800 $\pm$ 0.0423 & 0.6491 $\pm$ 0.1796 \\ \cline{2-5} 
          & Numerai         & 0.0214 $\pm$ 0.0004 & 1.3209 $\pm$ 0.0291 & 0.6607 $\pm$ 0.3372 \\ \hline
\multirow{3}{*}{2}   & No          & 0.0257 $\pm$ 0.0005 & 1.3457 $\pm$ 0.0431 & 0.3194 $\pm$ 0.0996 \\ \cline{2-5} 
          & XGB         & 0.0239 $\pm$ 0.0002 & 1.3486 $\pm$ 0.0334 & 0.4271 $\pm$ 0.1621 \\ \cline{2-5} 
          & Numerai         & 0.0196 $\pm$ 0.0006 & 1.2422 $\pm$ 0.0588 & 0.3783 $\pm$ 0.1300 \\ \hline
\multirow{3}{*}{3}   & No          & 0.0266 $\pm$ 0.0005 & 1.4116 $\pm$ 0.0372 & 0.3322 $\pm$ 0.0358 \\ \cline{2-5} 
          & XGB         & 0.0237 $\pm$ 0.0006 & 1.4279 $\pm$ 0.0445 & 0.4536 $\pm$ 0.1201 \\ \cline{2-5} 
          & Numerai         & 0.0200 $\pm$ 0.0007 & 1.2824 $\pm$ 0.0521 & 0.6315 $\pm$ 0.1521 \\ \hline
\multirow{3}{*}{4}   & No          & 0.0267 $\pm$ 0.0002 & 1.3427 $\pm$ 0.0281 & 0.2250 $\pm$ 0.0224 \\ \cline{2-5} 
          & XGB         & 0.0247 $\pm$ 0.0008 & 1.3574 $\pm$ 0.0502 & 0.2688 $\pm$ 0.0552 \\ \cline{2-5} 
          & Numerai         & 0.0205 $\pm$ 0.0003 & 1.2256 $\pm$ 0.0161 & 0.2993 $\pm$ 0.0533 \\ \hline
\multirow{3}{*}{5}   & No          & 0.0262 $\pm$ 0.0006 & 1.3398 $\pm$ 0.0480 & 0.3806 $\pm$ 0.0764 \\ \cline{2-5} 
          & XGB         & 0.0245 $\pm$ 0.0011 & 1.3380 $\pm$ 0.0570 & 0.5238 $\pm$ 0.1487 \\ \cline{2-5} 
          & Numerai         & 0.0204 $\pm$ 0.0006 & 1.2102 $\pm$ 0.0524 & 0.6052 $\pm$ 0.1681 \\ \hline
\multirow{3}{*}{6}   & No          & 0.0263 $\pm$ 0.0004 & 1.3625 $\pm$ 0.0347 & 0.2218 $\pm$ 0.0263 \\ \cline{2-5} 
          & XGB         & 0.0241 $\pm$ 0.0008 & 1.3985 $\pm$ 0.0194 & 0.2722 $\pm$ 0.0712 \\ \cline{2-5} 
          & Numerai         & 0.0199 $\pm$ 0.0006 & 1.2172 $\pm$ 0.0323 & 0.3377 $\pm$ 0.0774 \\ \hline
\multirow{3}{*}{7}   & No          & 0.0261 $\pm$ 0.0005 & 1.3371 $\pm$ 0.0332 & 0.2892 $\pm$ 0.0429 \\ \cline{2-5} 
          & XGB         & 0.0251 $\pm$ 0.0005 & 1.4207 $\pm$ 0.0526 & 0.4943 $\pm$ 0.1674 \\ \cline{2-5} 
          & Numerai         & 0.0207 $\pm$ 0.0003 & 1.2295 $\pm$ 0.0325 & 0.5921 $\pm$ 0.0934 \\ \hline
\multirow{3}{*}{8}   & No          & 0.0265 $\pm$ 0.0005 & 1.3851 $\pm$ 0.0207 & 0.3134 $\pm$ 0.0626 \\ \cline{2-5} 
          & XGB         & 0.0261 $\pm$ 0.0010 & 1.5093 $\pm$ 0.0547 & 0.7271 $\pm$ 0.2437 \\ \cline{2-5} 
          & Numerai         & 0.0205 $\pm$ 0.0005 & 1.2549 $\pm$ 0.0236 & 0.4790 $\pm$ 0.1051 \\ \hline
\multirow{3}{*}{9}   & No          & 0.0264 $\pm$ 0.0005 & 1.3912 $\pm$ 0.0474 & 0.2573 $\pm$ 0.0523 \\ \cline{2-5} 
          & XGB         & 0.0235 $\pm$ 0.0008 & 1.4067 $\pm$ 0.0328 & 0.4717 $\pm$ 0.1206 \\ \cline{2-5} 
          & Numerai         & 0.0204 $\pm$ 0.0002 & 1.2714 $\pm$ 0.0306 & 0.5578 $\pm$ 0.1206 \\ \hline
\multirow{3}{*}{10}  & No          & 0.0251 $\pm$ 0.0002 & 1.2942 $\pm$ 0.0229 & 0.2638 $\pm$ 0.0539 \\ \cline{2-5} 
          & XGB         & 0.0226 $\pm$ 0.0004 & 1.2669 $\pm$ 0.0490 & 0.3002 $\pm$ 0.0557 \\ \cline{2-5} 
          & Numerai         & 0.0195 $\pm$ 0.0001 & 1.1688 $\pm$ 0.0152 & 0.5257 $\pm$ 0.0734 \\ \hline
\end{tabular}
\smallskip
    \caption{Performance of standard XGBoost Models with different feature sampling schemes and feature projection schemes (No: No feature projection, XGB: Bad features based on XGBoost feature importance, Numerai: fixed set of 416 features given by Numerai) on validation period (Eras 601-885)}
    \label{table:XGBFeatureStandard-validate}
\end{table}

\begin{table}[]
\begin{tabular}{|c|c|l|l|l|}
\hline
Feature Set         & Projection  & Mean Corr & Sharpe & Calmar \\ \hline
\multirow{3}{*}{1}  & No           & 0.0276 $\pm$ 0.0002 & 1.4516 $\pm$ 0.0107 & 0.3675 $\pm$ 0.0292 \\ \cline{2-5} 
        & XGB        & 0.0268 $\pm$ 0.0002 & 1.5215 $\pm$ 0.0194 & 0.5855 $\pm$ 0.0803 \\ \cline{2-5} 
        & Numerai        & 0.0224 $\pm$ 0.0002 & 1.3643 $\pm$ 0.0118 & 0.6354 $\pm$ 0.0511 \\ \hline
\multirow{3}{*}{2}  & No           & 0.0267 $\pm$ 0.0001 & 1.3942 $\pm$ 0.0114 & 0.3534 $\pm$ 0.0396 \\ \cline{2-5} 
        & XGB        & 0.0253 $\pm$ 0.0005 & 1.4031 $\pm$ 0.0497 & 0.3942 $\pm$ 0.0756 \\ \cline{2-5} 
        & Numerai        & 0.0210 $\pm$ 0.0001 & 1.3090 $\pm$ 0.0122 & 0.4432 $\pm$ 0.0510 \\ \hline
\multirow{3}{*}{3}  & No           & 0.0282 $\pm$ 0.0001 & 1.4910 $\pm$ 0.0143 & 0.4774 $\pm$ 0.0431 \\ \cline{2-5} 
        & XGB        & 0.0256 $\pm$ 0.0002 & 1.4717 $\pm$ 0.0201 & 0.6196 $\pm$ 0.0857 \\ \cline{2-5} 
        & Numerai        & 0.0217 $\pm$ 0.0002 & 1.3844 $\pm$ 0.0174 & 0.7209 $\pm$ 0.0972 \\ \hline
\multirow{3}{*}{4}  & No           & 0.0279 $\pm$ 0.0001 & 1.4051 $\pm$ 0.0044 & 0.3078 $\pm$ 0.0102 \\ \cline{2-5} 
        & XGB        & 0.0268 $\pm$ 0.0003 & 1.4640 $\pm$ 0.0230 & 0.3193 $\pm$ 0.0143 \\ \cline{2-5} 
        & Numerai        & 0.0218 $\pm$ 0.0002 & 1.2959 $\pm$ 0.0128 & 0.3204 $\pm$ 0.0219 \\ \hline
\multirow{3}{*}{5}  & No           & 0.0273 $\pm$ 0.0002 & 1.4213 $\pm$ 0.0178 & 0.5537 $\pm$ 0.0640 \\ \cline{2-5} 
        & XGB        & 0.0266 $\pm$ 0.0002 & 1.4373 $\pm$ 0.0184 & 0.5935 $\pm$ 0.1229 \\ \cline{2-5} 
        & Numerai        & 0.0214 $\pm$ 0.0002 & 1.2889 $\pm$ 0.0100 & 0.6559 $\pm$ 0.0747 \\ \hline
\multirow{3}{*}{6}  & No           & 0.0276 $\pm$ 0.0001 & 1.4616 $\pm$ 0.0132 & 0.3060 $\pm$ 0.0305 \\ \cline{2-5} 
        & XGB        & 0.0256 $\pm$ 0.0005 & 1.4294 $\pm$ 0.0345 & 0.3538 $\pm$ 0.0675 \\ \cline{2-5} 
        & Numerai        & 0.0212 $\pm$ 0.0001 & 1.2715 $\pm$ 0.0073 & 0.3972 $\pm$ 0.0319 \\ \hline
\multirow{3}{*}{7}  & No           & 0.0271 $\pm$ 0.0002 & 1.4215 $\pm$ 0.0135 & 0.3920 $\pm$ 0.0183 \\ \cline{2-5} 
        & XGB        & 0.0270 $\pm$ 0.0005 & 1.4795 $\pm$ 0.0375 & 0.3453 $\pm$ 0.0520 \\ \cline{2-5} 
        & Numerai        & 0.0221 $\pm$ 0.0002 & 1.3147 $\pm$ 0.0200 & 0.7696 $\pm$ 0.1224 \\ \hline
\multirow{3}{*}{8}  & No           & 0.0276 $\pm$ 0.0000 & 1.4667 $\pm$ 0.0119 & 0.3955 $\pm$ 0.0486 \\ \cline{2-5} 
        & XGB        & 0.0277 $\pm$ 0.0003 & 1.6234 $\pm$ 0.0217 & 1.1689 $\pm$ 0.1616 \\ \cline{2-5} 
        & Numerai        & 0.0219 $\pm$ 0.0001 & 1.3533 $\pm$ 0.0158 & 0.6421 $\pm$ 0.0684 \\ \hline
\multirow{3}{*}{9}  & No           & 0.0282 $\pm$ 0.0002 & 1.5239 $\pm$ 0.0223 & 0.3850 $\pm$ 0.0531 \\ \cline{2-5} 
        & XGB        & 0.0255 $\pm$ 0.0003 & 1.5326 $\pm$ 0.0312 & 0.4746 $\pm$ 0.0321 \\ \cline{2-5} 
        & Numerai        & 0.0219 $\pm$ 0.0002 & 1.3262 $\pm$ 0.0167 & 0.4133 $\pm$ 0.0336 \\ \hline
\multirow{3}{*}{10} & No           & 0.0263 $\pm$ 0.0001 & 1.3789 $\pm$ 0.0162 & 0.3534 $\pm$ 0.0492 \\ \cline{2-5} 
        & XGB        & 0.0246 $\pm$ 0.0005 & 1.3848 $\pm$ 0.0319 & 0.2858 $\pm$ 0.0383 \\ \cline{2-5} 
        & Numerai        & 0.0207 $\pm$ 0.0001 & 1.2550 $\pm$ 0.0109 & 0.4735 $\pm$ 0.037  \\ \hline
\end{tabular}
\smallskip
    \caption{Performance of large XGBoost Models with different feature sampling schemes and feature projection schemes (No: No feature projection, XGB: Bad features based on XGBoost feature importance, Numerai: fixed set of 416 features given by Numerai) on validation period (Eras 601-885)}
    \label{table:XGBFeatureLarge-validate}
\end{table}

%%%% Comparision with Meta Model

\paragraph{Compare with Meta Model} 
\begin{table}[]
\begin{tabular}{|c|c|l|l|l|}
\hline
Meta Model &  & 0.0207 & 1.0073 & 0.3492   \\ \hline
\multirow{2}{*}{Small}  & original    & 0.0240 $\pm$ 0.0003 & 1.0511 $\pm$ 0.0223 & 0.3344 $\pm$ 0.0090 \\ \cline{2-5}
                        & ensemble  & 0.0262 $\pm$ 0.0001 & 1.1398 $\pm$ 0.0111 & 0.4576 $\pm$ 0.0190 \\ \hline
\multirow{2}{*}{Standard} & original      & 0.0247 $\pm$ 0.0002 & 1.0447 $\pm$ 0.0156 & 0.3921 $\pm$ 0.0629 \\ \cline{2-5}
                        & ensemble  & 0.0259 $\pm$ 0.0002 & 1.1202 $\pm$ 0.0091 & 0.4759 $\pm$ 0.0153 \\\hline
\multirow{2}{*}{Large}  & original      & 0.0251 $\pm$ 0.0001 & 1.0723 $\pm$ 0.0053 & 0.4426 $\pm$ 0.0301 \\ \cline{2-5}
                        & ensemble  & 0.0262 $\pm$ 0.0002 & 1.1348 $\pm$ 0.0036 & 0.4720 $\pm$ 0.0133 \\ \hline
\end{tabular}
\smallskip
    \caption{Performance of (a) small, (b) standard and (c) large XGBoost Models with different model complexity and data sampling schemes on test period  (Eras 901-1050), compared with Meta Model along with equal weighted ensemble of Meta Model and itself.}
    \label{table:XGBComplexityMeta}
\end{table}

\begin{table}[]
\begin{tabular}{|c|c|l|l|l|l|l|l|}
\hline
Meta Model &  & 0.0207  & 1.0073 & 0.3492  \\ \hline
\multirow{2}{*}{Small}  & original     & 0.0232 $\pm$ 0.0005 & 1.1238 $\pm$ 0.0167 & 0.2251 $\pm$ 0.0072 \\ \cline{2-5} 
                        & ensemble & 0.0251 $\pm$ 0.0002 & 1.1658 $\pm$ 0.0121 & 0.3528 $\pm$ 0.0098 \\ \hline
\multirow{2}{*}{Standard} & original     & 0.0237 $\pm$ 0.0002 & 1.1434 $\pm$ 0.0165 & 0.3454 $\pm$ 0.0410 \\ \cline{2-5} 
                        & ensemble & 0.0257 $\pm$ 0.0001 & 1.1891 $\pm$ 0.0099 & 0.4318 $\pm$ 0.0095 \\ \hline
\multirow{2}{*}{Large}  & original     & 0.0235 $\pm$ 0.0003 & 1.1505 $\pm$ 0.0248 & 0.4147 $\pm$ 0.0350 \\ \cline{2-5} 
                        & ensemble & 0.0260 $\pm$ 0.0001 & 1.2114 $\pm$ 0.0050 & 0.4838 $\pm$ 0.0062 \\ \hline
\end{tabular}
\smallskip
    \caption{Performance of (a) small, (b) standard and (c) large XGBoost Models with different feature sampling schemes on test period  (Eras 901-1050), compared with Meta Model along with equal weighted ensemble of Meta Model and itself.}
    \label{table:XGBFeatureMeta}
\end{table}

%%% Unused Background materials 

\subsection{Gradient Boosting Models} 

Gradient Boosting Decision Trees is a standard tool for tabular data modelling. There are many efficient implementations, for example, XGBoost \cite{XGBoost}, LightGBM \cite{LightGBM} and CatBoost \cite{CatBoost}. In this paper, XGBoost is used as it offers good GPU acceleration and flexible feature sub-sampling at the node level. 

\paragraph{Gradient Boosting Algorithm} 

Gradient Boosting is a generic algorithm for combining base learners in a sequential manner to obtain better predictions. A common choice of base learners would be decision trees. The aim of (gradient) boosting is to reduce \textbf{bias} of the ensemble learner. The aim is different to that of bagging, which fits multiple independent base learners at the same time, and the ensemble learner has a lower \textbf{variance} than each base learner. For practical implementations, bagging and boosting can often be used together. For example, in XGBoost, multiple trees (forests) can be fit in each boosting round. However empirical experience (as shown in textbooks like \cite{pml1Book}) suggests boosting works better than bagging for most datasets. Therefore, only a single tree is trained in each boosting round for the gradient boosting models used in this study. Algorithm \ref{alg:gradient-boosting} shows the pseudo-code for the general gradient boosting for a regression problem. 

\begin{algorithm}[htb!]
Given $N$ data samples $(\mathbf{x_i}, y_i), 1 
\leq i \leq N$ with the aim to find an increasing better estimate $\hat{f}(\mathbf{x})$ of the minimising function $f(x)$ which minimise the loss $\mathcal{L}(f)$ between targets and predicted values. $\mathcal{L}(f) = \sum_i l(y_i,f(\mathbf{x_i})) $ where $l$ is a given loss function such as mean square losses for regression problems. Function $f$ is restricted to the class of additive models $f(\mathbf{x}) = \sum_{k=1}^K w_k h(\mathbf{x},	\bm{\alpha_k})$ where $h(\cdot,\bm{\alpha})$ is a weak learner with parameters $\bm{\alpha}$ and $w_k$ are the weights. \\

Initialise  $f_0(\mathbf{x}) = \arg \min_{\bm{\alpha_0}} \sum_{i=1}^N l(y_i, h(\mathbf{x_i}, 	\bm{\alpha_0}))$  \\

\For{k = 1 : K}{
    Compute the gradient residual using $g_{ik} = - \left [ \frac{\partial l(y_i, f_{k-1}(\mathbf{x_i})) }{\partial f_{k-1}(\mathbf{x_i}) } \right ]  $ \\
    Use the weak learner to compute $\bm{\alpha_k}$ which minimises $ \sum_{i=1}^N (g_{ik} - h(\mathbf{x_i},	\bm{\alpha_k}))^2 $  \\
    Update with learning rate $\lambda$ $f_k(\mathbf{x}) = f_{k-1}(\mathbf{x}) + \lambda h(\mathbf{x}, \bm{\alpha_k}) $ \\ 
}
\textbf{Return} $f(\mathbf{x}) = f_K(\mathbf{x})$ \\
\caption{Gradient boosting algorithm \cite{FriedmanJeromeH.2001GfaA, B_hlmann_2007} }
\label{alg:gradient-boosting}
\end{algorithm}

\subsection{Detailed results of XGBoost model snapshots in validation period}

\begin{table}[!ht]
 (a) Small XGBoost models (Max Boosting rounds = 500, Learning rate = 0.1)
\begin{center}
    \begin{tabular}{|l|l|l|l|l|l|l|}
    \hline
    Complexity & Mean Corr  & Sharpe & Calmar \\ \hline
    0.1        & 0.0189    $\pm$ 0.0012    & 0.9611 $\pm$ 0.0567 & 0.1951 $\pm$ 0.0486 \\ \hline
    0.2        & 0.0215    $\pm$ 0.0005    & 1.0681 $\pm$ 0.0201 & 0.2311 $\pm$ 0.0583 \\ \hline
    0.3        & 0.0222    $\pm$ 0.0009    & 1.1115 $\pm$ 0.0471 & 0.3132 $\pm$ 0.151  \\ \hline
    0.4        & 0.0229    $\pm$ 0.001     & 1.1852 $\pm$ 0.0659 & 0.4139 $\pm$ 0.1599 \\ \hline
    0.5        & 0.0235    $\pm$ 0.0004    & 1.2405 $\pm$ 0.0264 & 0.4275 $\pm$ 0.0795 \\ \hline
    0.6        & 0.0237    $\pm$ 0.0008    & 1.2458 $\pm$ 0.0582 & 0.4707 $\pm$ 0.1168 \\ \hline
    0.7        & 0.0236    $\pm$ 0.0009    & 1.2608 $\pm$ 0.053  & 0.5006 $\pm$ 0.1628 \\ \hline
    0.8        & 0.0235    $\pm$ 0.0014    & 1.2741 $\pm$ 0.108  & 0.634  $\pm$ 0.246  \\ \hline
    0.9        & 0.0238    $\pm$ 0.0012    & 1.2884 $\pm$ 0.0872 & 0.6521 $\pm$ 0.266  \\ \hline
    1.0        & 0.0238    $\pm$ 0.0011    & 1.3169 $\pm$ 0.0874 & 0.6336 $\pm$ 0.239  \\ \hline
    \end{tabular}
 %   \label{table:XGBSnapshot1}
  %       \caption{Model Snapshots of small XGBoost Models (Max Boosting rounds is 500, Learning rate is 0.1) between 2014-07-04 (Era 601) and 2018-04-27 (Era 800)}
\end{center}
\bigskip
(b) Standard XGBoost models (Max Boosting rounds = 5000, Learning rate = 0.01)
\begin{center}
 %   \caption{Model Snapshots of standard XGBoost Models (Max Boosting rounds is 5000, Learning rate is 0.01) between 2014-07-04 (Era 601) and 2018-04-27 (Era 800)}
    \begin{tabular}{|l|l|l|l|l|l|l|}
    \hline
    Complexity & Mean Corr & Sharpe & Calmar \\ \hline
    0.1        & 0.0217    $\pm$ 0.0001    & 1.0521 $\pm$ 0.0075 & 0.2257 $\pm$ 0.0193 \\ \hline
    0.2        & 0.0245    $\pm$ 0.0002    & 1.1831 $\pm$ 0.0175 & 0.3117 $\pm$ 0.0371 \\ \hline
    0.3        & 0.0259    $\pm$ 0.0003    & 1.2688 $\pm$ 0.0212 & 0.3901 $\pm$ 0.0621 \\ \hline
    0.4        & 0.0268    $\pm$ 0.0002    & 1.3311 $\pm$ 0.0253 & 0.4423 $\pm$ 0.0674 \\ \hline
    0.5        & 0.0276    $\pm$ 0.0003    & 1.3807 $\pm$ 0.0345 & 0.52   $\pm$ 0.1134 \\ \hline
    0.6        & 0.0281    $\pm$ 0.0002    & 1.4149 $\pm$ 0.0286 & 0.6229 $\pm$ 0.1546 \\ \hline
    0.7        & 0.0284    $\pm$ 0.0003    & 1.4409 $\pm$ 0.0391 & 0.7143 $\pm$ 0.1777 \\ \hline
    0.8        & 0.0285    $\pm$ 0.0004    & 1.4536 $\pm$ 0.0418 & 0.7891 $\pm$ 0.1685 \\ \hline
    0.9        & 0.0285    $\pm$ 0.0005    & 1.4656 $\pm$ 0.0512 & 0.8137 $\pm$ 0.1077 \\ \hline
    1.0        & 0.0285   $\pm$ 0.0004    & 1.4695 $\pm$ 0.0439 & 0.8141 $\pm$ 0.0882 \\ \hline
    \end{tabular}
%    \label{table:XGBSnapshot2}
\end{center}
\bigskip
(c) Large XGBoost models (Max Boosting rounds = 50000, Learning rate = 0.001)
\begin{center}
%    \caption{Model Snapshots of large XGBoost Models (Max Boosting rounds is 50000, Learning rate is 0.001) between 2014-07-04 (Era 601) and 2018-04-27 (Era 800)}
    \begin{tabular}{|l|l|l|l|l|l|l|}
    \hline
    Complexity & Mean Corr & Sharpe & Calmar \\ \hline
    0.1        & 0.0221    $\pm$ 0.0001    & 1.0685 $\pm$ 0.0067 & 0.2424 $\pm$ 0.0067 \\ \hline
    0.2        & 0.0249    $\pm$ 0.0001    & 1.1926 $\pm$ 0.0079 & 0.327  $\pm$ 0.0148 \\ \hline
    0.3        & 0.0262    $\pm$ 0.0001    & 1.2743 $\pm$ 0.0082 & 0.3928 $\pm$ 0.0173 \\ \hline
    0.4        & 0.0271    $\pm$ 0.0001    & 1.3334 $\pm$ 0.0072 & 0.4445 $\pm$ 0.0304 \\ \hline
    0.5        & 0.0277    $\pm$ 0.0001    & 1.3776 $\pm$ 0.0089 & 0.51   $\pm$ 0.0335 \\ \hline
    0.6        & 0.0282    $\pm$ 0.0001    & 1.4151 $\pm$ 0.0091 & 0.5884 $\pm$ 0.0468 \\ \hline
    0.7        & 0.0285    $\pm$ 0.0001    & 1.4422 $\pm$ 0.0107 & 0.6638 $\pm$ 0.0531 \\ \hline
    0.8        & 0.0288    $\pm$ 0.0001    &  1.462  $\pm$ 0.0092 & 0.7726 $\pm$ 0.0825 \\ \hline
    0.9        & 0.0288    $\pm$ 0.0001    & 1.4747 $\pm$ 0.0063 & 0.8925 $\pm$ 0.1111 \\ \hline
    1.0        & 0.0289    $\pm$ 0.0001    & 1.4839 $\pm$ 0.0084 & 1.0072 $\pm$ 0.1164 \\ \hline
    \end{tabular}
\end{center}
\smallskip
    \caption{Performance of (a) small, (b) standard and (c) large XGBoost Models of different complexity on validation period  (Eras 601-800)}
    \label{table:XGBSnapshots}
\end{table}
